# Supplementary material for: Dominant Shuffle: A Simple Yet Powerful Data Augmentation for Time-series Prediction
Source: arXiv:2405.16456 source file (2024-05-26)
Supplement: Supplementary file 1 [file long_term_3models_eth_appendix.tex]

\multirow{11}{*}{\makecell{Auto \\ former \\ ~\cite{wu2021autoformer}}} & Baseline& \base{0.429} & \base{0.440} & \base{0.495} & \base{0.498} & \base{0.381} & \base{0.443} & \base{0.471} & \base{0.475} & \base{0.467} & \base{0.610} & \base{0.529} & \base{0.773} \\%& \base{0.233} & \base{0.278} & \base{0.383} & \base{0.488}  \\
& ASD & 0.450 & 0.485 & 0.523 & 0.556 & 0.370 & 0.465 & 0.476 & 0.503  & 0.480 & 0.620 & 0.502 & 0.633\\
& MSB & 0.462&0.517& 0.612 & 0.579 &0.434 & 0.523 & 0.556 & 0.462 & 0.499 & 0.645 & 0.553 & 0.721 \\
& Upsample & 0.416 & 0.523 & 0.480 & 0.482 & 0.353 & 0.460 & 0.455 & 0.509 & 0.498 & 0.630 & 0.512& 0.667\\
& FreqAdd & 0.460 & 0.487 & 0.497 & 0.525 & 0.367 & 0.439 & 0.480 & 0.504 & 0.419 & 0.554 & 0.546 & 0.569 \\
& FreqPool &\\
& Robusttad &\\
& STAug & 0.429 & 0.478 & 0.505 & 0.506 & 0.354 & 0.443 & 0.496 & 0.495 & 0.415 & 0.581 & 0.588 & 0.693\\
& Mask & 0.424 & 0.468 & 0.485 & \best{0.474} & 0.363 & 0.424 & 0.470 & 0.467 & 0.459 & 0.510 & \best{0.491} & 0.588 \\%& 0.217 & 0.267 & 0.347 & 0.451 \\
& Mix & 0.420 & 0.445 & 0.467 & 0.523 & 0.358 & 0.421 & 0.480 & 0.505 & 0.415 & 0.566 & 0.503 & 0.610 \\%& 0.211 & 0.274 & 0.340 & 0.461 \\
& Ours& \best{0.409} & \best{0.436} & \best{0.458} & 0.486 & \best{0.335} & \best{0.419} & \best{0.453} & \best{0.452} & \best{0.392} & \best{0.506} & \best{0.491} & \best{0.559} \\%& \best{0.210} & \best{0.266} & \best{0.329} & \best{0.429} \\
\hline
\multirow{11}{*}{\makecell{MICN \\ ~\cite{wang2023micn}}} & Baseline& \base{0.384} & \base{0.425} & \base{0.464} & \base{0.574} & \base{0.358} & \base{0.518} & \base{0.566} & \base{0.827} & \base{0.313} & \base{0.360} & \base{0.389} & \base{0.461} \\%& \base{0.200} & \base{0.282} & \base{0.375} & \base{0.606}  \\
& ASD &0.380&0.430&0.472&0.523&0.377&0.539&0.620&0.843&0.315&0.362&0.399&0.357\\
& MSB &0.423&0.421&0.501&0.559&0.402&0.623&0.790&1.126&0.330&0.358&0.402&0.459\\
& Upsample &0.396&0.435&0.463&0.550&0.366&0.500&0.831&0.752&0.339&0.377&0.402&0.475\\
& FreqAdd & 0.390 & 0.430 & 0.477 & 0.643 & 0.370 & 0.521 & 0.626 & 0.975 & 0.316 & 0.360 & 0.407 & 0.478\\
& FreqPool &\\
& Robusttad &\\
& STAug & 0.374 & 0.429 & 0.489 & 0.608 & 0.413 & 0.760 & 1.33 & 2.608 & 0.313 & 0.360 & 0.418 & 0.483 \\
& Mask & 0.381 & 0.424 & 0.460 & 0.543 & 0.339 & 0.489 & 0.544 & 0.735 & 0.309 & 0.360 & 0.407 & 0.475 \\%& 0.184 & 0.265 & 0.353 & 0.510 \\
& Mix & 0.378 & 0.423 & 0.461 & 0.521 & 0.339 & 0.488 & 0.562 & 0.767 & \best{0.301} & \best{0.352} & 0.401 & \best{0.454} \\%& 0.183 & 0.278 & 0.356 & 0.528 \\
& Ours& \best{0.373} & \best{0.421} & \best{0.452} & \best{0.510} & \best{0.310} & \best{0.427} & \best{0.507} & \best{0.731} & 0.314 & 0.360 & \best{0.387} & 0.470 \\%& \best{0.174} & \best{0.263} & \best{0.346} & \best{0.502} \\
\hline
\multirow{11}{*}{Lightts} & Baseline& \base{0.448} & \base{0.444} & \base{0.663} & \base{0.706} & \base{0.369} & \base{0.476} & \base{0.738} & \base{1.165} & \base{0.323} & \base{0.347} & \base{0.428} & \base{0.476} \\%& \base{0.212} & \base{0.237} & \base{0.350} & \base{0.473}  \\
& ASD &0.451&0.476&0.633&0.681&0.392&0.469&0.701&0.998&0.356&0.352&0.441&0.478\\
& MSB &0.467&0.463&0.627&0.652&0.378&0.472&0.652&1.123&0.371&0.349&0.430&0.479\\
& Upsample &0.449&0.472&0.610&0.637&0.401&0.487&0.714&1.245&0.329&0.366&0.453&0.492\\
& FreqAdd & 0.417 & 0.430 & 0.578 & 0.622 & 0.351 & 0.453 & 0.689 & 1.125 & 0.322 &0.352&0.400&0.450\\
& FreqPool &\\
& Robusttad &\\
& STAug & 0.445 & 0.441 & 0.669 & 0.714 & 0.520 & 0.807 & 2.101 & 2.467 & 0.320 & 0.343 & 0.427 & 0.476\\
& Mask & 0.418 & 0.432 & 0.573 & 0.621 & 0.339 & 0.447 & 0.643 & 0.993 & 0.324 & 0.342 & 0.400 & 0.449 \\%& 0.204 & 0.238 & 0.321 & 0.435 \\
& Mix & 0.417 & 0.429 & 0.575 & 0.620 & 0.337 & 0.426 & 0.650 & 1.046 & \best{0.316} & \best{0.340} & 0.398 & 0.447 \\%& 0.199 & \best{0.233} & 0.322 & 0.440 \\
& Ours& \best{0.405} & \best{0.423} & \best{0.565} & \best{0.603} & \best{0.335} & \best{0.395} & \best{0.575} & \best{0.827} & 0.322 & \best{0.340} & \best{0.391} & \best{0.440}
