# Supplementary material for: Dominant Shuffle: A Simple Yet Powerful Data Augmentation for Time-series Prediction
Source: arXiv:2405.16456 source file (2024-05-26)
Supplement: Supplementary file 2 [file long_term_3models_weather_appendix.tex]

% long-term 3 models weather datasets appendix
